# Supplementary material for: Searching for polarization in signed graphs: a local spectral approach
Source: arXiv:2001.09410 source file (2020-01-26)
Supplement: Supplementary file 2 [file appendix_implementation_details.tex]

\section{Algorithmic details}
\label{sec:impl}

We first describe how to find $\xopt = \betaopt \pinv{\lap - \alphaopt \dmat} \dmat \vs$ without knowing the value of $\alphaopt$ beforehand\footnote{Note that once $\alphaopt$ is found, the value $\betaopt$ can be computed by normalizing $\pinv{\lap - \alphaopt \dmat} \dmat \vs$ with respect to $\dmat$.}.

Then, we give a procedure that rounds the real-valued vector \vxopt to $(\Sone, \Stwo)$ which minimizes $\sbr(\Sone, \Stwo)$. 

\subsection{Finding $\xopt$ efficiently}

First, given $\alphaopt$, $\pinv{\lap - \alphaopt \dmat}$  can be approximated using Conjugate Gradient Method~\cite{golub2012matrix} in time $\bigO({m \sqrt{c}})$, where $c$ is the condition number of $\lap - \alphaopt \dmat $.

Then we use complementary slackness condition $(\vxopt)^T (\dmat \vs)(\dmat \vs)^T \vxopt = \kappa$ (Condition~\ref{eq:cs1})
and apply binary search on $\alpha \in [-\vol(\graph), \eigval)$. 
The search stops when $\vx^T (\dmat \vs)(\dmat \vs)^T \vx$ is close enough to $\kappa$.

\subsection{Efficient rounding of $\xopt$ to $(\Sone, \Stwo)$}
\label{sec:fast-sweep}
By Proposition 1, we use threshold $t \in \real^{+}$ to round the solution from $\vx$ to $(\Sone(t), \Stwo(t))$, where
$\Sone(t) = \nodes_{\vx}(t) = \set{u \in \nodes \mid {\vx}(u) \ge t}$ and $\Stwo(t) = \nodes_{\vx}(-t) = \set{u \in \nodes \mid {\vx}(u) \le -t}$. 
And we select $t$ that minimizes $\sbr(\Sone(t), \Stwo(t))$.
As a convention, when we say ``order'', we refer to descending order by default. 
We describe how to find the optimal $t$ in $\bigO(m+n+n\log(n))$, where $n\log(n)$ is the cost of sorting a vector.  

\paragraph{An equivalent problem.}
First, it's easy to see that we only need to evaluate $t$ values from the set $\domain(\vx) = \set{\abs{\vx(i)} \mid i=1,\ldots,n}$ and $\abs{\domain(\vx)} \le n$. 
Without loss of generality, we assume $\avx$ is strictly ordered,
e.g., $\avx(i) > \avx(i+1)$, for all $i=1, \ldots, n-1$. 
In other words, thresholding on $t=\avx(i)$ takes the top-$i$ nodes ordered by $\avx$.
We denote these nodes as $\Cavx[i]$.
Similar, we define the top-$i$ nodes ordered by $\vx$ and $\nvx$ as
$\Cvx[i]$ and $\Cnvx[i]$ respectively. 

Further, we decompose $\Cavx[i]$ into two disjoint sets $\Cvx[j]$ and $\Cnvx[k]$,
where the values of $j$ and $k$ implicitly depend on $\Cavx[i]$ and $\vx$, 
e.g., $j =\abs{\set{u \in \Cavx[i] \mid \vx_u \ge 0}}$
and $k =\abs{\set{u \in \Cavx[i] \mid \vx_u < 0}}$. 
It immediately follows that $j+k \le i$. 

Thus, the problem of

\begin{align*}
  t^{*} &= \argmin_{t \in \domain(\vx)} \sbr(\Sone(t), \Stwo(t)) \\
        &= \argmin_{t \in \domain(\vx)} \frac{2\abs{\posedges(\Sone(t), \Stwo(t))} +  \abs{\negedges(\Sone(t))} + \abs{\negedges(\Stwo(t))} + \abs{\edges(\Sone(t)\cup\Stwo(t), \nodes\setminus(\Sone(t)\cup\Stwo(t)))}}{\vol(\Sone(t) \cup \Stwo(t))}
\end{align*}

given \vx, is equivalent to:

\[
  i^{*} = \argmin_{i \in \set{1,\ldots,n}}
  \frac{2\abs{\posedges(\Cvx[j], \Cnvx[k])} + 
    \abs{\negedges(\Cvx[j])} + \abs{\negedges(\Cnvx[k])} + 
    \abs{\edges(\Cavx[i], \nodes\setminus \Cavx[i])}}{\vol(\Cavx[i])}.
\]

where $j$ and $k$ are implicitly determined by the choice $i$.
Finally,  $t^{*}=\avx(i^{*})$. 

Our algorithm evaluates at all possible $i$ and pick the optimal position.
It achieves efficiency by re-using intermediate results. 
Specifically, we compute the related terms at $i$ e.g., $\abs{\posedges(\Cvx[j], \Cnvx[k])}$ from terms at $1,\ldots,i-1$ that are \textit{already} computed. 

Next, we show how to compute each term separately in $\bigO(m+n)$.

\paragraph{Computing $\vol(\Cavx[\cdot])$. }
We define the \textit{\vx-ordered volume}, $\vol_\vx$, which is affected by node ordering induced by $\vx \in \real^{n}$. 
The $i$th element, $\vol_\vx[i]$ equals the summation of the degrees of top-$i$ nodes ordered by \vx.
As a naming convention, we use subscript terms to indicate the ordering, which gives more variants, e.g, $\vol_{\nvx}[i]$ and $\vol_{\avx}[i]$.
We also consider signed counterparts of \vx-ordered volume, e.g.,
$\posvol_{\vx}[i]$ and $\negvol_{\vx}[i]$. 

Then, we have the following equivalence for all $i=1,\ldots,n$:

\[
  \vol(\Cavx[i]) = \vol_{\avx}[i] 
\]

$\vol_{\avx}[\cdot]$ can be computed incrementally by the following recursion in $\bigO(m+n)$:

\[
  \vol_{\avx}[i] = \vol_{\avx}(i-1) + \degree(i)
\]

for all $i=1,\ldots,n$ and $\vol_{\avx}[0]=0$. 

In a similar fashion, we can compute: 
$\posvol_{\vx}$, $\posvol_{\nvx}$, $\negvol_{\vx}$, $\negvol_{\nvx}$ and $\negvol_{\avx}$, in $\bigO(m+n)$.

\paragraph{Computing $\abs{\edges(\Cavx[\cdot], \nodes\setminus\Cavx[\cdot])}$.}
As a short-cut, we write $\cut_{\avx}[i] = \abs{\edges(\Cavx[i], \nodes\setminus\Cavx[i])}$ and similarly,
$\poscut_{\avx}[i] = \abs{\posedges(\Cavx[i], \nodes\setminus\Cavx[i])}$ and
$\negcut_{\avx}[i] = \abs{\negedges(\Cavx[i], \nodes\setminus\Cavx[i])}$.

We will use the following matrices to compute $\poscut_{\avx}[i]$ and $\negcut_{\avx}[i]$. 
$\Lp$ and $\Ln$ are the lower triangular matrix of $\Ap$ and $\An$ respectively. 
Given a vector $\vx \in \real^{n}$ and a matrix $M \in \real^{n \times n}$,
we define $M_\vx$ as the \textit{$\vx$-ordered matrix $M$}. 
$M_\vx$ equals $M$ with both rows and columns permuted by the ordering induced by $\vx$.
Using this notation, we have the corresponding matrices on $\Ap$ and $\An$ with rows and columns permuted by the $\vx, \nvx, \text{ or } \avx$.

We define $\posin_\vx[i]$ (resp. $\negin_\vx[i]$) as the number of positive (resp. negative) edges in the subgraph induced by top-$i$ nodes from the ordering by $\vx$.
Formally, we have the following recursion computable in $\bigO(m+n)$:

\begin{align*}
  \posin_\avx[i] &= \posin_\avx(i-1) + 2\;\sum_{j=1}^n\Lp_\avx(i, j) \\
  \negin_\avx[i] &= \negin_\avx(i-1) + 2\;\sum_{j=1}^n\Ln_\avx(i, j)
\end{align*}

And

\begin{align*}
  \poscut_\avx[i] &= \posvol_\avx[i] - \posin_\avx[i] \\
  \negcut_\avx[i] &= \negvol_\avx[i] - \negin_\avx[i] 
\end{align*}

Obviously, $\cut_{\avx}[i]=\poscut_{\avx}[i] + \negcut_{\avx}[i]$.
Therefore, $\cut_\avx[i]$ can be computed in $\bigO(m+n)$. 

\paragraph{Computing $\abs{\negedges(\Cvx[j])} + \abs{\negedges(\Cnvx[k])}$ given $\vx$ and $i$. }
For brevity, we denote $\negin_{\vx}(\cdot) = \abs{\negedges(\Cvx[\cdot])}$
and similarly, $\negin_{\nvx}(\cdot) = \abs{\negedges(\Cnvx[\cdot])}$. 
Both $\negin_{\vx}(\cdot)$ and $\negin_{\vx}(\cdot)$ can be computed in $\bigO(m+n)$ as shown previously.

Recall that $j$ and $k$ are determined implicitly:
$j =\abs{\set{u \in \Cavx[i] \mid \vx_u \ge 0}}$
and $k = i-j$ respectively.
In practice, given $[i]_1^n$, the corresponding list of $[j]$ and $[k]$ can be computed in $\bigO(n)$.

Therefore, $\negin_{\vx}(j) + \negin_{-\vx}(k)$ can be aggregated in $\bigO(m+n)$ for all $i=\enlst{1}{n}$. 

\paragraph{Computing $\abs{\posedges(\Cvx[j], \Cnvx[k])}$. }
We use the following observation:

\[
  \posedges(\Cvx[j], \Cnvx[k]) = \posedges(\Cvx[j], \nodes\setminus\Cvx[j]) \cup \posedges(\Cnvx[k], \nodes\setminus\Cnvx[k]) \setminus \posedges(\Cavx[i], \nodes\setminus\Cavx[i])
\]

It follows immediately:

\[
  \abs{\posedges(\Cvx[j], \Cnvx[k])} = \poscut_\vx[j] + \poscut_{\nvx}[k] - \poscut_\avx[i]
\]

Therefore, $\abs{\posedges(\Cvx[j], \Cnvx[k])}$ can be computed in $\bigO(m+n)$ for all $i=\enlst{1}{n}$.
