# Supplementary material for: Searching for polarization in signed graphs: a local spectral approach
Source: arXiv:2001.09410 source file (2020-01-26)
Supplement: Supplementary file 4 [file supplementary.tex]

\documentclass{article}

% if you need to pass options to natbib, use, e.g.:
%     \PassOptionsToPackage{numbers, compress}{natbib}
% before loading neurips_2018

% ready for submission
% \usepackage{neurips_2018}

% to compile a preprint version, e.g., for submission to arXiv, add add the
% [preprint] option:
%     \usepackage[preprint]{neurips_2018}

% to compile a camera-ready version, add the [final] option, e.g.:
\usepackage[final]{nips_2018}

% to avoid loading the natbib package, add option nonatbib:
%     \usepackage[nonatbib]{neurips_2018}

\usepackage[utf8]{inputenc} % allow utf-8 input
\usepackage[T1]{fontenc}    % use 8-bit T1 fonts
\usepackage{hyperref}       % hyperlinks
\usepackage{url}            % simple URL typesetting
\usepackage{booktabs}       % professional-quality tables
\usepackage{amsfonts}       % blackboard math symbols
\usepackage{nicefrac}       % compact symbols for 1/2, etc.
\usepackage{microtype}      % microtypography
\usepackage{amsmath}
\usepackage{amssymb}
\usepackage{mathtools}
\usepackage{natbib}
\usepackage{graphicx}
\usepackage{url}
\usepackage{xspace}
\usepackage{float}
\usepackage{tikz}
\usetikzlibrary{calc,positioning}
\usepackage{varwidth}

\usepackage{amsthm}
\usepackage[ruled, vlined, nofillcomment, linesnumbered]{algorithm2e}

\input{defines}

\title{Supplementary material}

% The \author macro works with any number of authors. There are two commands
% used to separate the names and addresses of multiple authors: \And and \AND.
%
% Using \And between authors leaves it to LaTeX to determine where to break the
% lines. Using \AND forces a line break at that point. So, if LaTeX puts 3 of 4
% authors names on the first line, and the last on the second line, try using
% \AND instead of \And before the third author name.

\author{%\\
  % examples of more authors
  % \And
  % Coauthor \\
  % Affiliation \\
  % Address \\
  % \texttt{email} \\
  % \AND
  % Coauthor \\
  % Affiliation \\
  % Address \\
  % \texttt{email} \\
  % \And
  % Coauthor \\
  % Affiliation \\
  % Address \\
  % \texttt{email} \\
  % \And
  % Coauthor \\
  % Affiliation \\
  % Address \\
  % \texttt{email} \\
}

\begin{document}
% \nipsfinalcopy is no longer used

\maketitle

\begin{abstract}
\end{abstract}

\input{main_results}
\input{proof}
\input{proof2}

\subsubsection*{Acknowledgments}

Use unnumbered third level headings for the acknowledgments. All acknowledgments
go at the end of the paper. Do not include acknowledgments in the anonymized
submission, only in the final paper.

\section*{References}
\bibliographystyle{plain}
\bibliography{references}

\end{document}
